# Supplementary material for: Fast, Anytime Motion Planning for Prehensile Manipulation in Clutter
Source: arXiv:1806.07465 source file (2019-02-11)
Supplement: Supplementary file 1 [file appendix_0.tex]

\subsection{FFEE JK-PRM* Idea 1}

The general idea is to create an FFEE roadmap where the connectivity is based off of
the capability of the arm to jac-steer from one config to another.  For each reachable
ffee config (reachable since it was an FK of an arm state), we attempt to jac steer to 
all other ffee configs.  Each jac steer should be seeded with a different IK solution of
the current config, and we keep track of how many successes there have been.  We repeat
this process for the same pair of ffee configs a number of times before moving on to computing
the rank for the next config in the list. This then
allows us to then rank the other configs in the list based off of jac-steering success rate,
and we can then base our connectivity

\begin{algorithm}[]
\caption{FFEE JK PRM}
\label{algo:FFEE_JK_PRM}
Sample $N$ random arm states: $\mathbf{X}_{rand}$ \\
Compute the end-effector configurations: $\mathbf{Q}_{rand} \leftarrow \mathtt{FK}(\mathbf{X}_{rand})$ \\
\For{$q_i, q_j \in \mathbf{Q}_{rand} \land i \neq j$}
{
    $rank(q_i, q_j) \leftarrow \mathtt{COMPUTE\_RANK}(q_i,q_j)$ \\
    $\mathbf{R({q_i})} \leftarrow \mathbf{R({q_i})} \cup \{rank(q_i, q_j)\}$ \\
    Sort $\mathbf{R({q_i})}$ \\
    Connect $q_i$ to k-best sorted configs \\
 }

\end{algorithm}

\begin{algorithm}[]
\caption{$\mathtt{COMPUTE\_RANK}(q_i,q_j)$}
\label{algo:compute_rank}
$JK_{+} \leftarrow 0$ \\
\For{$q_j \in \mathbf{Q}_{rand} \land i \neq j$}
{
    $I \leftarrow \mathtt{NUM\_IK\_ATTEMPTS}$ \\
    \While{$I > 0 $}
    {
        $x_{q_i} \leftarrow \mathtt{IK}(q_i)$ \\
        \If{ $x_{q_i} \emph{is\_valid}$ }
        {
            \If{ $\mathtt{JK\_STEER}(x_{q_i}, q_j) \emph{is\_valid}$}
            {
                $JK_{+} \leftarrow JK_{+} + 1$
            }
        }
        $I \leftarrow I - 1$
    }
}

\textbf{return}$\ JK_{+}  $\;

\end{algorithm}

\subsection{Evaluating the effects of clutter on various steering methods}

The purpose of this section to study the effects of clutter on three different
steering methods for manipulator: local steering, IK-steering, and Jacobian-steering.
The purpose of these steering methods is to generate a trajectory for the manipulator
given an initial manipulator state $x_{s}$ and a target end-effector
pose $q_{g}$.

{\textbf{Local steering}:} refers to taking a straight line interpolation in the configuration
space of the manipulator from $x_{s}$ to the IK-solution of the end-effector pose $q_{g} \rightarrow x_g$ and 
generating a corresponding trajectory using the maximum velocity bounds of the manipulator's joints. 

{\textbf{IK-steering}:} refers to taking a straight line interpolation in the end-effector space (SE3) from
the FK of $x_{s} \rightarrow q_{s}$ to $q_g$, using the maximum velocity bounds of the end-effector.
These bounds can be estimated by {\textbf{local steering}} to many different pairs of ${x_s,q_g}$,
and keeping track of the velocity of the end-effector in each of these trajectories.  Along the
SE3 interpolation $q_s \rightarrow q_g$, we generate a trajectory by calling IK on each consecutive pair of
configurations (seeded with the previous iteration's solutions) and then {\textbf{local steering}} between these two IK
solutions.

{\textbf{Jacobian steering}:} refers to computing the damped least-squares (DLS) pseudo-inverse Jacobian for from
the initial manipulator state $x_s$ to the goal configuration $q_g$.  During this process, we apply clamping
over the controls to ensure that they remain within the bounds of the manipulator.

{\textbf{Preprocessing}:} In order to evaluate these steering methods, a certain amount of preprocessing must occur first. The preprocessing
is to ensure the following: first, that the tests do not inherently introduce any bias into the statistics (such
as from the choice of the end-effector); second, that each steering method is evaluated on the same dataset;
and finally that the dataset changes in a uniform and measurable fashion - specifically, with regards to
the amount of free space available to the robot (approximately measured as volume in the sphere of reachability
of the manipulator).
\begin{enumerate}
    \item{Ensure the URDF is for a single arm, with no end-effector attached.}
    \item{Generate scenes with an increasing percent of obstacles in the volume of the reachable workspace.}
    \item{Sample $n$-collision free arm states, and save these in the set $\mathbf{X_{free}}$.}
    \item{Sample $k$-reachable end-effector poses, and save these in the set $\mathbf{Q_{reachable}}$}
    \item{Generate $m$ state and pose evaluation pairs $(x',q'), x' \in \mathbf{X_{free}}, q' \in \mathbf{Q_{reachable}} $}
\end{enumerate}

Specifically for generating the $m$ evaluation pairs. Sample a random state $x_{rand} \in \mathbf{X_{free}}$.  Compute
$q_{rand} \leftarrow FK(x_{rand})$ and find the $l$ nearest-neighbors from $\mathbf{Q_{reachable}}$.  Here $l$ is chosen
to be roughly $0.25 * |\mathbf{Q_{reachable}}|$, of which we select $j << l$ random samples from it. The reason for this process
is to ensure that the steering methods are not attempting to reach configurations which are too far away, while simultaneously
ensuring that we are not only evaluating steering to configurations which are very close.

{\textbf{Evaluation}:} The process for evaluating the steering methods online is fairly straight forward. For each evaluation
pair $(x_i, q_i)$, we invoke the corresponding steering method and measure the following metrics.
\begin{enumerate}
    \item{{\textbf{Steering Success}}: Whether the method could compute an IK or Jacobian to the goal.}
    \item{{\textbf{Computation Time}}: The amount of time the method needed to compute the trajectory to the goal, or report failure. }
    \item{{\textbf{Path Length}}: The summed pairwise distances in the trajectory measured in configuration space. }
    \item{{\textbf{End-Effector Displacement}}: The summed pairwise C-DIST costs in the trajectory. }
\end{enumerate}
